# Supplementary material for: Imaging dynamic exciton interactions and coupling in transition metal dichalcogenides
Source: arXiv:2202.09089 ancillary file (2022-02-18)
Supplement: Supplementary file 1 [file HS_Imaging_SI_v1.pdf]

# Imaging dynamic exciton interactions and coupling in transition metal dichalcogenides - Supplementary information

Torben L. Purz,<sup>1</sup> Eric W. Martin,<sup>2</sup> William G. Holtzmann,<sup>3</sup> Pasqual Rivera,<sup>3</sup> Adam Alfrey,<sup>1</sup> Kelsey M. Bates,<sup>1</sup> Hui Deng,<sup>1</sup> Xiaodong Xu,<sup>3</sup> and Steven T. Cundiff<sup>1,\*</sup>

<sup>1</sup>*Department of Physics, University of Michigan, Ann Arbor MI 48109-1040, USA*

<sup>2</sup>*MONSTR Sense Technologies LLC, Ann Arbor MI 48104, USA*

<sup>3</sup>*Department of Physics, University of Washington, Seattle, WA 98195-1560, USA*

(Dated: February 7, 2022)

## MDCS SCHEME AND EXPERIMENTAL SETUP

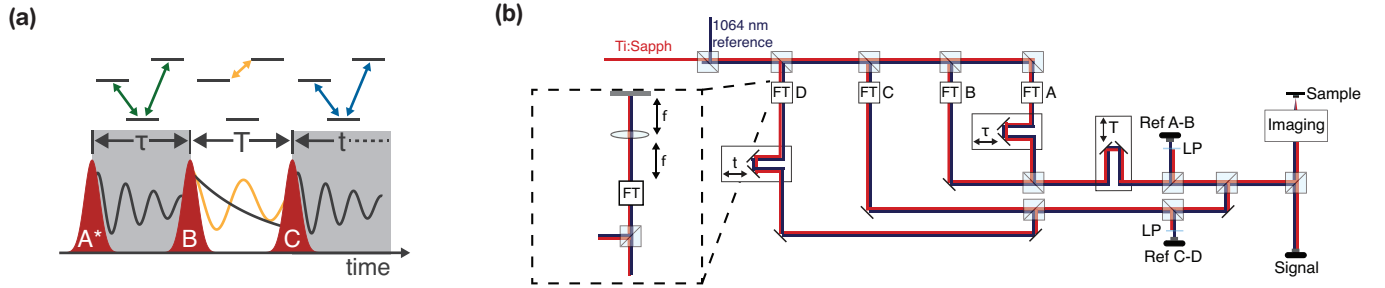

FIG. S1. (a) Scheme for one-quantum rephasing MDCS. (b) Schematic drawing of the MDCIS setup used to obtain the data presented in the main text and supplemental information

The multi-dimensional coherent spectroscopy (MDCS) scheme for the one-quantum rephasing pathway [1] at the heart of this work is shown in Fig. S1(a). The system is in a coherence between ground and excited state during  $\tau$  (green arrow) and  $t$  (blue arrow), which are scanned and Fourier transformed. During  $T$ , the system can be in either a population or Raman-like non-radiative coherence (yellow arrow) between two excited states in the same manifold. The latter manifests itself as a decaying oscillation during  $T$ , as demonstrated in Fig. 5 and 6 in the main text.

The experimental setup, with an emphasis on the spectroscopy part of the setup is shown in Fig. S1(b). The laser-scanning based imaging setup omitted here is shown in Fig. 1(d) in the main text. The sample is cooled to 5 K using an Advanced Research Systems (ARS) closed cycle cryostat. Pulses from the Coherent Vitara laser (variable bandwidth and center wavelength) coming into the setup are chirp pre-compensated to durations within 20% of the transform limit (measured at the sample). Pre-compensation is realized with a homebuilt pulse shaper, employing a Meadowlark Linear Series Spatial Light Modulator ( $1 \times 12,288$  pixels). Beams are frequency-tagged using acousto-optics modulators (Isomet 1205-C). As illustrated in the dashed box in Fig. S1(b), the acousto-optic modulators are double passed to cancel spatial chirp. All three beams generating the signal (A,B,C) and the fourth beam used for heterodyne detection (D) are subsequently recombined and focused onto the sample using a long working distance objective (Nikon 20x, NA=0.4). The four-wave-mixing (FWM) signal and beams reflected from the sample are detected on a silicon variable gain detector (New Focus, Model 2117-FS). The detected signal is sent to a lock-in amplifier (MONSTR Sense Technologies). All four beams are co-propagated by a 50 mW, 1064 nm Nd:Yag Laser (CrystaLaser) which references path length changes between A-B and C-D. The signal from this reference is used to calculate the FWM reference for lock-in detection.

\* cundiff@umich.edu

## LINEWIDTH FITS

### A. Fitting scheme in temporal and frequency domain

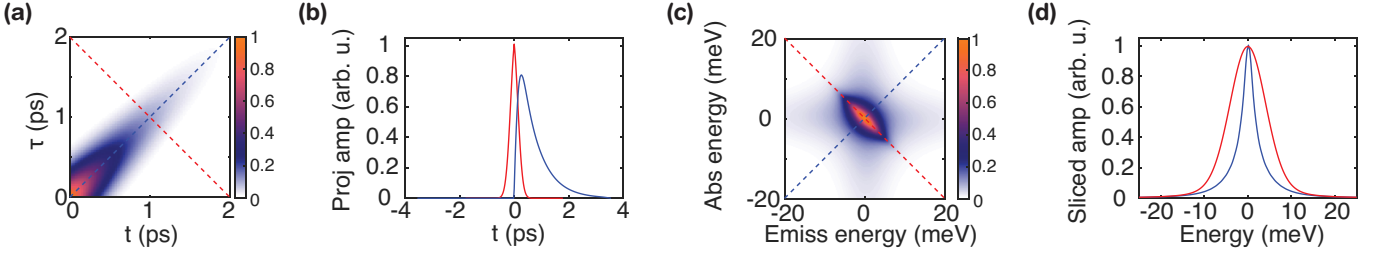

FIG. S2. (a) Time-trace for an MDCS measurement, showing the characteristic photon echo. (b) Projection onto the diagonal (blue) and cross-diagonal (red) drawn in (a). (c) MDCS spectrum obtained by Fourier transform of the time-trace in (a). (d) Slices along the diagonal (red) and cross-diagonal (blue) drawn in (c).

The fitting procedure based on the analytical analysis of Siemens *et al.* [2] is illustrated in Fig. S2. A typical time-domain signal for MDCS is shown in Fig. S2(a), with the photon-echo shape suggesting the existence of inhomogeneity. The homogeneous and inhomogeneous linewidth of the signal can be extracted either in the temporal, or the frequency domain. For linewidth extraction in the temporal domain, projections onto the diagonal (blue-dashed line in Fig. S2(a)) and the cross-diagonal (red-dashed line in Fig. S2(a)), as plotted in Fig. S2(b) can be used. The analytical form of the projections in the temporal domain for arbitrary inhomogeneity can be found in Eqs. (10) and (12) of Ref.[2]. An alternative treatment can be realized in the frequency domain, where instead of projections, slices along the diagonal (red-dashed line in Fig. S2(c)) and cross-diagonal (blue-dashed line in Fig. S2(c)) are taken. The corresponding slices are plotted in Fig. S2(d) and the corresponding analytical equations for the lineshapes can be found in Eqs. (11) and (13) of [2]. The two methods are direct Fourier transform equivalents of each other.

### B. Advantage of frequency over time-domain fitting

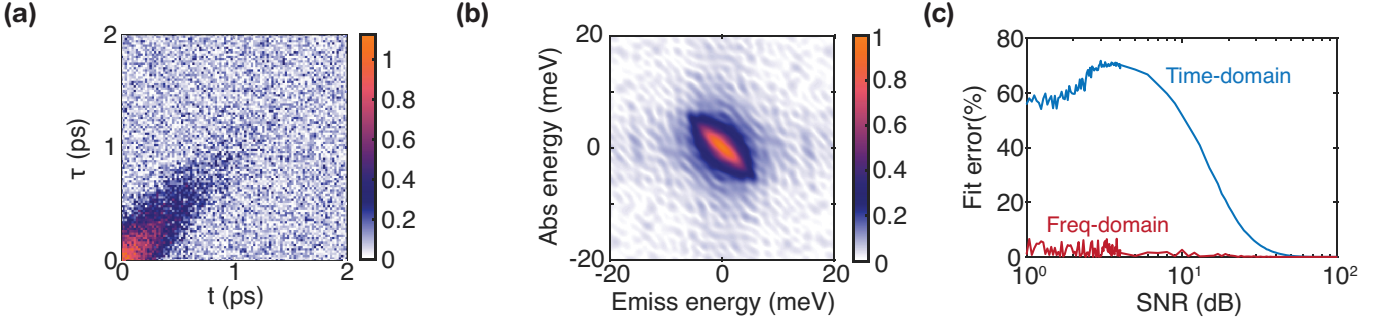

FIG. S3. (a) Time-trace for an MDCS measurement with an SNR of 20 dB. (b) Corresponding MDCS spectrum (c) Fit error as a function of SNR for both frequency-domain slice, and time-domain projection fits.

While in the ideal, noise-free scenario these two fitting procedures are equivalent, the advantage of the frequency domain fitting procedure becomes quickly apparent once noise is considered. The time-domain trace of the same signal as in Fig. S2, but with a signal-to-noise ratio (SNR) of 0 dB is shown in Fig. S3. Projecting onto the diagonal and cross-diagonal to extract the linewidths will evidently lead to a significant noise contribution that yields a large error on the extracted linewidths. In the simulation here, we use white Gaussian noise to model the experimental noise. This is a valid assumption since our experiments are limited by the shot noise of the DC background, wherefore we are able to obtain Fellgett's advantage, since the noise is still signal independent [3]. Given the nature of the noise, the Fourier-transformed MDCS spectrum plotted in Fig. S3(b) shows a significantly higher SNR. The fit error in the frequency domain is further reduced because instead of projections, only slices are taken, wherefore only the high signal region contributes.

It should be noted that the considerations above are only true for 2D-Fourier transform spectroscopy where the data is fully acquired in the temporal domain. Mixed-time-frequency domain spectroscopies as e.g. employed by [4, 5] are more prone to noise since only one Fourier transform (either into the time domain or frequency domain) is performed. The aspect of slices in the frequency domain being dominated by high signal contributions while noise has a considerable influence for the projections in the temporal domain however still remains true. Obtaining linewidths fits in the temporal and frequency domain for a myriad of SNR values, we plot the fit error as a function of SNR in Fig. S3(c). Both time and frequency domain show noticeable fit errors for low SNR, though the frequency-domain fit error never exceeds 10%. Moreover, the frequency domain error reaches acceptable levels of several percent and below around a SNR of 4 dB, while the time-domain error only reaches these levels around 35 dB. In conclusion, the frequency-domain fitting allows for much more robust retrieval of linewidths even for low SNR and reaches very reliable results much sooner. This allows for faster, higher noise measurements with reasonable acquisition times, e.g. in multi-dimensional coherent imaging spectroscopy (MDCIS).

### C. Linewidth fitting and absorption correction

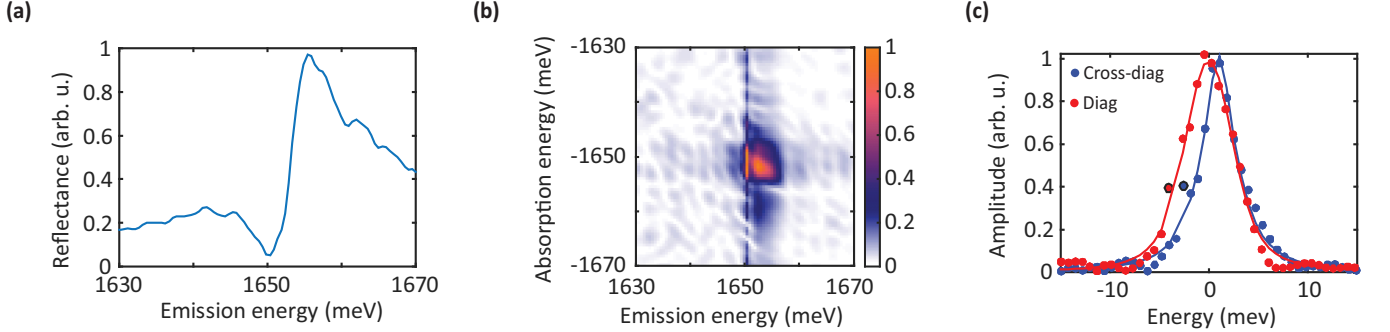

FIG. S4. **(a)** Reflectance spectrum for the MoSe<sub>2</sub> monolayer, showing a strong dip around 1650 meV. **(b)** Using the reflectance spectrum from (a) in the correction scheme leads to a singular line at fixed emission energy that is dominated by noise, while the rest of the MDCS spectrum is reconstructed reliably. **(c)** Fit of diagonal and cross-diagonal slices when excluding specific emission energies with low reflectance. Data points that are excluded in the fits have a black edge.

Since the fourth pulse (D) used for heterodyne detection is also sent onto the sample, the absorption has to be considered to retrieve the accurate spectral weight along the emission energy axis. Transition metal dichalcogenide (TMD) monolayers at cryogenic temperatures have strong absorption. Due to multiple reflections stemming from substrate and hexagonal Boron nitride (hBN) encapsulation, reflectance spectra with strong absorption dips as plotted in Fig. S4(a) can result. In this case, FWM signals around the reflectance dip will be noise dominated and the absorption correction procedure fails for small parts of the spectrum, as illustrated in Fig. S4(b). As evident from the spectrum, data points towards the left and the right of the sharp bright line at 1650 meV are reliable. Hence, excluding the erroneous data point(s) can yield robust fits that extract the homogeneous and inhomogeneous linewidths reliably. This is illustrated in Fig. S4(c), which shows the diagonal and cross-diagonal slices of the spectrum in Fig. S4(b), with all data points where the reflection amplitude falls below 7.5% of the maximum excluded (marked with a black edge). The fits (solid lines) match the data points well and the extracted linewidths can be trusted. We employ the described cutoff procedure for data points where the reflected spectrum has an amplitude below 7.5% for all linewidth fit maps in the main text. The value 7.5% has been determined as a reasonable cutoff by observing fit errors and reliability of extracted linewidths for cutoffs between 2.5% and 15%. The extracted linewidths were only sensitive for a few sample points, as shown in Fig. S5. The area marked with a green rectangle in Fig. S5(a) is the only area of the sample showing noticeable linewidth changes when changing the cutoff to 7.5% (Fig. S5(b)) and 15% (Fig. S5(c)).

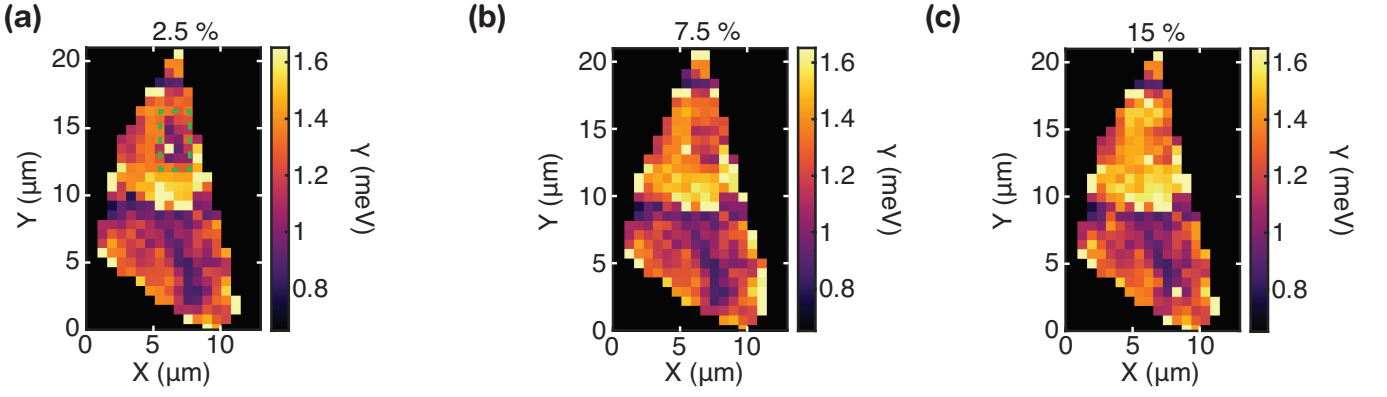

FIG. S5. Homogeneous linewidth ( $\gamma$ ) map of the MoSe<sub>2</sub> monolayer with a cutoff of (a) 2.5%, (b) 7.5%, (c) 15%.

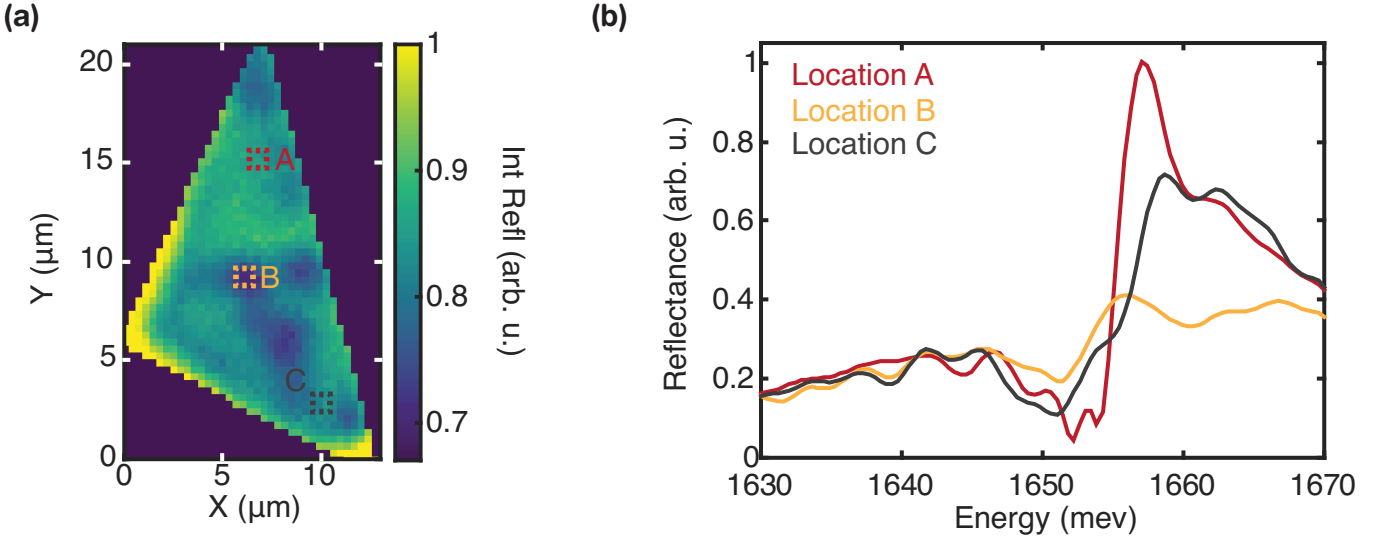

FIG. S6. (a) Integrated reflectance for the MoSe<sub>2</sub> monolayer. (b) Reflectance spectra for the three areas marked by colored squares in (a).

### LINEAR REFLECTANCE OF MOSE<sub>2</sub> MONOLAYER

The cutoff procedure described above is only crucial for a few select data points on the sample, as the reflectance spectrum varies strongly across the sample. The integrated reflectance map of the MoSe<sub>2</sub> monolayer sample is shown in Fig. S6(a). The high strain area of the sample identified in the main text shows a lower integrated reflectance. When plotting select spectra for the sample areas identified by the colored squares in Fig. S6(a), it is evident that the lower reflectance for the high strain, center area of the sample (yellow square) is due to an overall lower reflection, while for the two other sample areas selected here, the main difference lies in the depth of the reflectance dip around 1652 meV, as well as the height of the reflectance peak around 1657 meV. The stark differences can be explained by linewidth changes, which strongly influence the reflection coefficient for an encapsulated monolayer with numerous backreflections [6].

### LINEAR REFLECTANCE OF MOSE<sub>2</sub>/WSE<sub>2</sub> HETEROSTRUCTURE

The linear reflectance of the MoSe<sub>2</sub>/WSe<sub>2</sub> heterostructure shows strong changes towards the top of the sample, as illustrated by the integrated linear reflectance plotted in Fig. S7(a). Plotting select spectra for the sample areas identified by the colored squares in Fig. S7(a) in Fig. S7(b), it is evident that the higher integrated reflectance for the top of the sample (red square) stems from reduced absorption around the MoSe<sub>2</sub> resonance (1600-1630 meV), as well

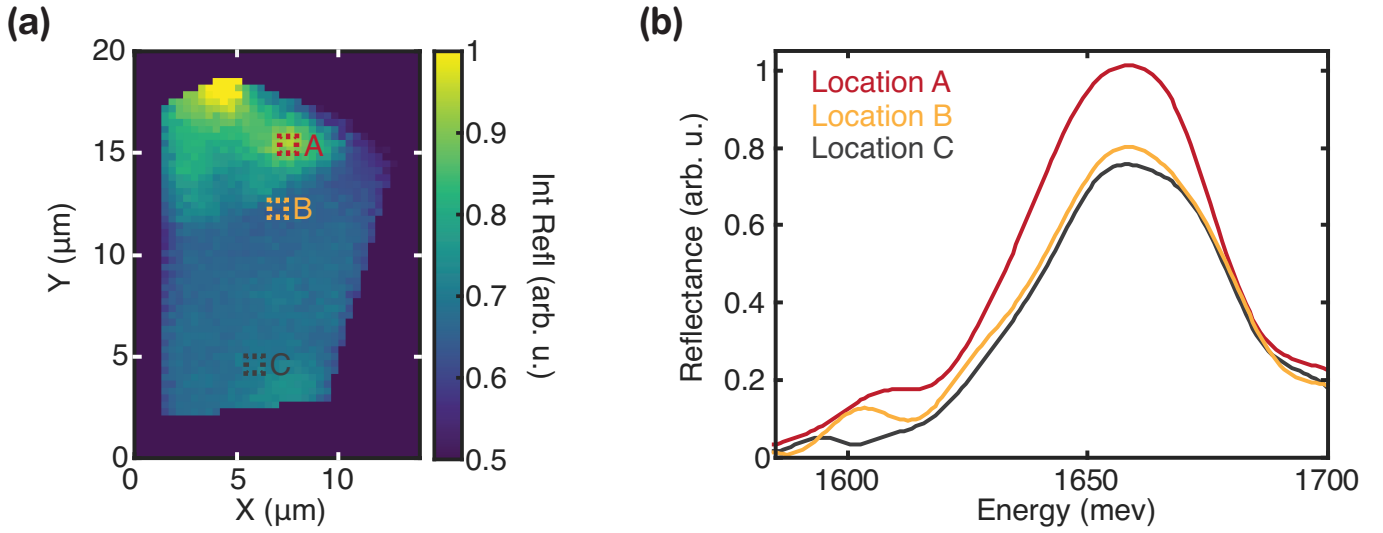

FIG. S7. (a) Integrated reflectance for the MoSe<sub>2</sub>/WSe<sub>2</sub> heterostructure. (b) Reflectance spectra for the three areas marked by colored squares in (a).

as a higher reflectance overall. The other two selected areas (yellow and gray square) show minor differences, with absorption and resonance energy for the MoSe<sub>2</sub> and WSe<sub>2</sub> varying as already discussed in the main text.

#### PL-DETECTED MDCS

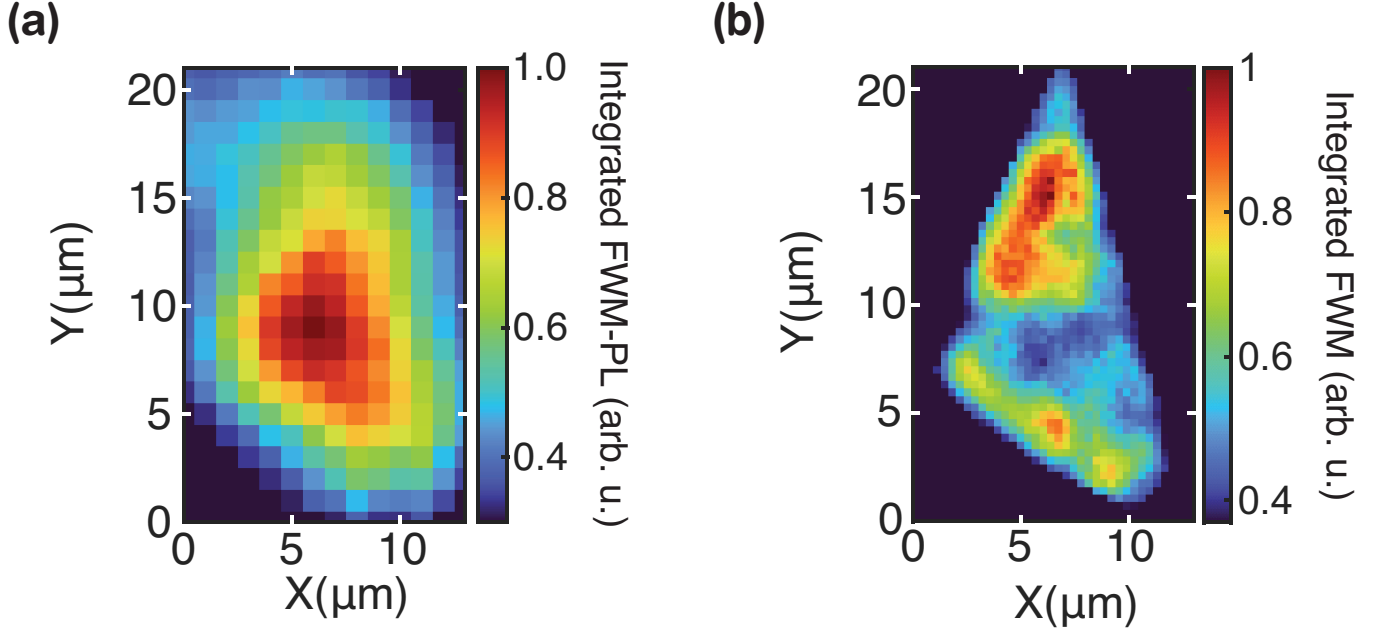

FIG. S8. (a) PL-detected FWM image of the MoSe<sub>2</sub> monolayer. (b) Heterodyne-detected FWM image of the MoSe<sub>2</sub> monolayer, same as Fig. 1(e) in the main text.

A comparison of photoluminescence (PL)-detected FWM imaging vs. heterodyne-detected FWM imaging is shown in Fig. S8. Fig. S8(a) shows the PL-detected FWM while Fig. S8(b) is the heterodyne-detected FWM from Fig. 1(e) in the main text. While the two figures have different spatial resolutions, mainly due to the 30° angle of the sample

in the PL-FWM setup (for details see [7]), it is evident that the low FWM area in Fig. S8(b) shows the highest FWM in Fig. S8(a). This can be traced back to the different distribution of bright and dark states and points towards a large number of dark states outside the center, high strain area of the monolayer.

- 
- [1] C. L. Smallwood and S. T. Cundiff, Multidimensional Coherent Spectroscopy of Semiconductors, *Laser & Photonics Reviews* **12**, 1800171 (2018).
  - [2] M. E. Siemens, G. Moody, H. Li, A. D. Bristow, and S. T. Cundiff, Resonance lineshapes in two-dimensional faourier transform spectroscopy, *Opt. Express* **18**, 17699 (2010).
  - [3] T. Hirschfeld, Fellgett's Advantage in uv-VIS Multiplex Spectroscopy, *Appl. Spectrosc.* **30**, 68 (1976).
  - [4] T. Jakubczyk, V. Delmonte, M. Koperski, K. Nogajewski, C. Faugeras, W. Langbein, M. Potemski, and J. Kasprzak, Radiatively limited dephasing and exciton dynamics in MoSe<sub>2</sub> monolayers revealed with four-wave mixing microscopy, *Nano Letters* **16**, 5333 (2016).
  - [5] A. D. Bristow, D. Karaiskaj, X. Dai, T. Zhang, C. Carlsson, K. R. Hagen, R. Jimenez, and S. T. Cundiff, A versatile ultrastable platform for optical multidimensional Fourier-transform spectroscopy, *Review of Scientific Instruments* **80**, 073108 (2009), <https://doi.org/10.1063/1.3184103>.
  - [6] H. H. Fang, B. Han, C. Robert, M. A. Semina, D. Lagarde, E. Courtade, T. Taniguchi, K. Watanabe, T. Amand, B. Urbaszek, M. M. Glazov, and X. Marie, Control of the Exciton Radiative Lifetime in van der Waals Heterostructures, *Phys. Rev. Lett.* **123**, 067401 (2019).
  - [7] K. M. Bates, M. W. Day, C. L. Smallwood, R. C. Owen, T. Schröder, E. Bielejec, R. Ulbricht, and S. T. Cundiff, Using silicon-vacancy centers in diamond to probe the full strain tensor, *Journal of Applied Physics* **130**, 024301 (2021), <https://doi.org/10.1063/5.0052613>.
